# Supplementary material for: A Computationally Efficient Learning-Based Model Predictive Control for Multirotors under Aerodynamic Disturbances
Source: arXiv:2402.10323 source file (2024-02-15)
Supplement: Supplementary file 1 [file appendix.tex]

\section*{APPENDIX}

Appendixes should appear before the acknowledgment.
